# Supplementary material for: Dynamic vorticity banding in discontinuously shear thickening suspensions
Source: arXiv:1802.10586 ancillary file (2018-11-25)
Supplement: Supplementary file 1 [file SI.pdf]

# Supplementary Material for "Dynamic vorticity banding in discontinuously shear thickening suspensions"

R. N. Chacko,[1] R. Mari,[2] M. E. Cates,[3] and S. M. Fielding[1]

[1] *Department of Physics, Durham University, Science Laboratories, South Road, Durham DH1 3LE, United Kingdom*

[2] *Univ. Grenoble Alpes, CNRS, LIPhy, 38000 Grenoble, France*

[3] *DAMTP, Centre for Mathematical Sciences, University of Cambridge, Wilberforce Road, Cambridge CB3 0WA, United Kingdom*

(Dated: June 13, 2018)

## FLOW SET UP

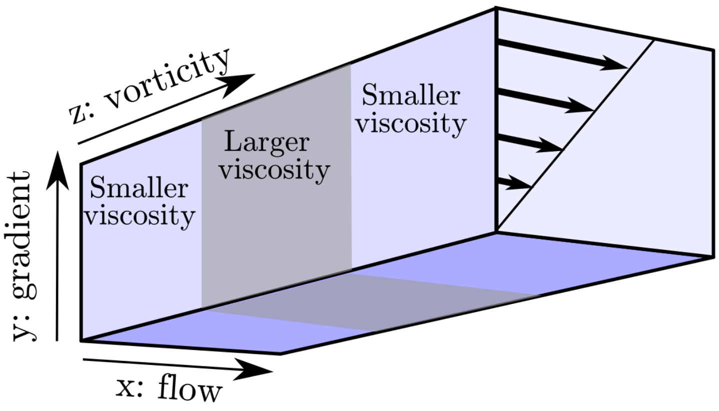


The system is under simple shear, with $x, y$ and $z$ respectively the flow, gradient and vorticity directions. The S-shaped $\sigma(\dot{\gamma})$ constitutive curve admits in principle coexistence of slices of the system sharing the same shear rate but having different shear viscosities, stacked along the vorticity direction.

## DETAILS OF THE TIME INTEGRATION OF THE CONTINUUM MODEL

The non-dimensionalised and re-scaled continuum simulation is solved using the forward Euler method on 512 gridpoints spaced regularly in $z$. Time-stepping due to local terms is done in real space, while that due to the Laplacian is done in Fourier space. Finally, while the time-step is initially set to $dt = 10^{-6}$, step-doubling (see [1], p.910) is used to determine the time-step during the evolution, with an error term $\epsilon := \max_{z_i \in \text{grid}} |\eta_2(z_i) - \eta_1(z_i)| / \langle\eta\rangle$, where the $\eta_2(z_i)$ is the viscosity at gridpoint $z_i$ after a single forward Euler step across a time interval $2\Delta t$ and $\eta_1$ is the viscosity at $z_i$ after two forward Euler steps, each across a time interval $\Delta t$. The upper limit of the allowed value of the error term is chosen so that halving the error tolerance does not change the $t \to \infty$ profiles. For TB states, we check this by shifting the final state in $z$ to get a best match between the two profiles, and for LOB states we check this by shifting in both $z$ and $t$.

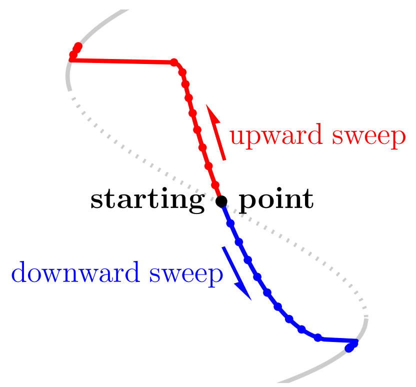


As seen in Fig. 2 (main text), there are values of $\bar{\sigma}/\sigma^*$ and $\bar{\phi}$ (e.g. $(\bar{\sigma}/\sigma^*, \bar{\phi}) = (10, 0.575)$) at which a TB state, an LOB state, and a homogeneous state are all stable $\gamma \to \infty$ solutions of the system. Linear stability analysis allows us to determine the full range of stable homogeneous states. For TB (LOB) states, we instead explore this range by slowly sweeping the stress up and down from an initially TB (LOB) steady state, as shown in the figure above. Specifically, a TB (LOB) flow curve is obtained by finding a system that has reached a steady TB (LOB) state, e.g. by perturbing an initially homogeneous system and evolving it in time, and using a snapshot of the $\sigma(z)$ and $\phi(z)$ profiles of the system in this state as a starting point for two separate stress sweeps, one increasing and one decreasing. Each sweep consists of a monotonic sequence of bulk stresses $(\bar{\sigma}_i)_i$, where at each $i$ a fixed $\bar{\sigma}_i$ is imposed and the system is evolved until the periodic limiting state is obtained. The initial $\sigma(z)$ and $\phi(z)$ profiles for the evolution at $\bar{\sigma}_{i+1}$ is then obtained as a snapshot of this limiting state. Finally, the full flow curve is obtained by stitching the flow curves from the upward and downward sweeps together.

## DETAILS OF THE TIME INTEGRATION OF THE PARTICLE-BASED MODEL

The numerical method of particle-based simulations has already been described in detail in [2] and [3]. The following section summarises that description in order to make the present paper self contained.

We simulate an assembly of inertialess frictional spheres immersed in a Newtonian fluid under simple shear flow. The system is binary, with radii $a$ and $1.4a$ mixed at equal volume fractions. Particles interact through hydrodynamic ($\boldsymbol{F}_{\mathrm{H}}$) and contact ($\boldsymbol{F}_{\mathrm{C}}$) forces. The equation of motion is the force balance between these forces which depend on the many-

body position and velocity vectors $\boldsymbol{X}$ and $\boldsymbol{U}(\equiv \dot{\boldsymbol{X}})$:

$$\mathbf{0} = \boldsymbol{F}_{\mathrm{H}}(\boldsymbol{X}, \boldsymbol{U}) + \boldsymbol{F}_{\mathrm{C}}(\boldsymbol{X}). \tag{1}$$

The hydrodynamic forces consist of two components, a drag due to the motion relative to the surrounding fluid, $-\boldsymbol{R}_{\mathrm{FU}}(\boldsymbol{X}) \cdot \big(\boldsymbol{U} - \boldsymbol{U}^{\infty}\big)$, and a resistance to the deformation imposed by the flow, $\dot{\gamma}\boldsymbol{R}_{\mathrm{FE}} : \hat{\boldsymbol{E}}^{\infty}$, where $\boldsymbol{U}_i^{\infty} = \dot{\gamma} y_i \hat{\boldsymbol{e}}_x$ and $\hat{\boldsymbol{E}}^{\infty} \equiv (\hat{\boldsymbol{e}}_x\hat{\boldsymbol{e}}_y + \hat{\boldsymbol{e}}_y\hat{\boldsymbol{e}}_x)/2$ is the normalized strain rate tensor. The resistance matrices $\boldsymbol{R}_{\mathrm{FU}}$ and $\boldsymbol{R}_{\mathrm{FE}}$ contain the Stokes drag and the leading terms of the pairwise hydrodynamic lubrication interaction regularized to mimic roughness and allow contacts [2, 4]. Regularization is achieved by inserting a small cutoff length scale $\delta$ [5], which can be thought of as the length scale of the particle surface roughness; the leading terms for lubrication forces we use for normal and tangential displacements then behave as $1/(h^{(i,j)} + \delta)$ and $\log(1/(h^{(i,j)} + \delta))$. We use $\delta = 10^{-3}$. Contacts are modeled by parallel linear spring and dashpot for the normal component, and spring alone for the tangential component giving rise to friction. The normal and tangential components of the force and the torque for particles having radii $a_i$ and $a_j$ are obtained as

$$\begin{aligned} \boldsymbol{F}_{\mathrm{C,nor}}^{(i,j)} &= k_{\mathrm{n}} h^{(i,j)} \boldsymbol{n}_{ij} + \gamma_{\mathrm{n}} \boldsymbol{U}_{\mathrm{n}}^{(i,j)}, \\ \boldsymbol{F}_{\mathrm{C,tan}}^{(i,j)} &= k_{\mathrm{t}} \boldsymbol{\xi}^{(i,j)}, \\ \boldsymbol{T}_{\mathrm{C}}^{(i,j)} &= a_i \boldsymbol{n}_{ij} \times \boldsymbol{F}_{\mathrm{C,tan}}^{(i,j)}, \end{aligned} \tag{2}$$

$k_{\mathrm{n}}$ and $k_{\mathrm{t}}$ are the normal and tangential spring constants, respectively, $\gamma_{\mathrm{n}}$ is the damping constant, $\boldsymbol{n}_{ij}$ is the center-to-center unit vector, $h^{(i,j)}$ is the normal spring stretch (overlap) and $\boldsymbol{\xi}^{(i,j)}$ is the tangential one. Crucially, contacts can bear a tangential force only when the normal force exceeds a threshold $F^{*}$ (the so-called "Critical Load Model" [2]), and when it does we use a Coulomb friction law with friction coefficient $\mu = 1$, i.e. $|\boldsymbol{F}_{\mathrm{C,tan}}^{(i,j)}| < \mu k_{\mathrm{n}} h^{(i,j)} - F^{*}$. We uses spring constants $k_{\mathrm{n}} = 5 \times 10^{3} \bar{\sigma} a$ and $k_{\mathrm{t}} = 0.5 k_{\mathrm{n}}$, which ensures that the maximum overlap between any two particles at any time during the simulation is around 4% of a particle radius for the values of applied stress $\bar{\sigma}$ explored in this work. Finally, we use $\gamma_{\mathrm{n}} = 10 \eta_0 a^3 \bar{\sigma}/F^{*}$, with $\eta_0$ the suspending fluid viscosity, ensuring that contact springs adapt to a change of load in roughly $10^{-4}$ strain units, that is, much faster than the microstruture response time $\gamma_0$.

The equation of motion (1) is completed by the constraint of flow at constant shear stress

$\bar{\sigma}$ [3]. At any time, the stress in the suspension is given by:

$$\sigma = \dot{\gamma}\eta_0\left(1 + \frac{5}{2}\phi\right) + \dot{\gamma}\eta_{\mathrm{E}} + \sigma_{\mathrm{C}} \tag{3}$$

with $\eta_0$ the suspending fluid viscosity, $\eta_{\mathrm{E}} = V^{-1}\left\{(\boldsymbol{R}_{\mathrm{SE}} - \boldsymbol{R}_{\mathrm{SU}} \cdot \boldsymbol{R}_{\mathrm{FU}}^{-1} \cdot \boldsymbol{R}_{\mathrm{FE}}) : \hat{\boldsymbol{E}}^{\infty}\right\}_{xy}$ and $\sigma_{\mathrm{C}} = V^{-1}\left(\boldsymbol{X}\boldsymbol{F}_{\mathrm{C}} - \boldsymbol{R}_{\mathrm{SU}} \cdot \boldsymbol{R}_{\mathrm{FU}}^{-1} \cdot \boldsymbol{F}_{\mathrm{C}}\right)_{xy}$, where $\boldsymbol{R}_{\mathrm{SU}}$ and $\boldsymbol{R}_{\mathrm{SE}}$ are resistance matrices giving the lubrication stresses from the particles' velocities and resistance to deformation, respectively [2, 6] and $V$ is the volume of the simulation box. At fixed shear stress $\bar{\sigma}$ the shear rate $\dot{\gamma}$ is the fluctuating variable that is to be determined at each time step by

$$\dot{\gamma} = \frac{\bar{\sigma} - \sigma_{\mathrm{C}}}{\eta_0\left(1 + 2.5\phi\right) + \eta_{\mathrm{E}}}. \tag{4}$$

The full solution of the equation of motion (1) under the constraint of fixed stress (3) is thus the following velocity $\boldsymbol{U}$:

$$\boldsymbol{U} = \boldsymbol{U}^{\infty}(\dot{\gamma}) + \boldsymbol{R}_{\mathrm{FU}}^{-1} \cdot \left(\dot{\gamma}\boldsymbol{R}_{\mathrm{FE}} : \hat{\boldsymbol{E}}^{\infty} + \boldsymbol{F}_{\mathrm{C}}\right). \tag{5}$$

We solve for this velocity at each time step to update the positions with a forward Euler scheme. The time increment $\Delta t$ is adapted at each time step such that the non-affine displacement $(\boldsymbol{U} - \boldsymbol{U}^{\infty})_i\Delta t$ for any particle $i$ is smaller than $10^{-3}a_i$.

## STRAIN FLUCTUATIONS AT CONTROLLED STRESS

In the continuum model, and in the particle-based simulations which are performed at controlled stress, the strain rate $\dot{\gamma}(t)$ remains uniform in space but fluctuates in time. Its time integral is the total strain, which we use instead of time as the ordinate in Fig. 3. This is convenient for experimental comparisons particularly in systems where aspects of the rheology are rate independent (in Wyart-Cates theory this applies to both the low-stress and the high-stress asymptotes where $f$ becomes constant, recovering rate-independent rheology). Indeed, the evolution of the microstructure in the model (and in the simulations) is controlled by a strain scale $\gamma_0$, not by a time scale.

In the particle-based simulations, the observed strain rate fluctuates around values of $2.6 \times 10^{-4}\sigma^*/\eta_{\mathrm{f}}$ for the top panel of Fig. 3 (TB state) and $2.5 \times 10^{-4}\sigma^*/\eta_{\mathrm{f}}$ for the bottom panel (LOB state). In the continuum model, for TB states past an initial transient, the strain rate does not fluctuate in steady state, which corresponds to a fixed profile that

simply shifts across a translationally invariant periodic box. LOB states however do have time-varying oscillating strain rates, with the same period than the one of the stress spatial profile, as mentioned in the main text.

Time series of the global strain rate $\dot{\gamma}(t)$ in TB (top row) and LOB (bottom row) regimes, for continuum (left column) and particle-based (right column) models are shown in the figure below. The data correspond to the spacetime plots shown in Fig. 3 of the main text. We see that, due to the modest flow-gradient dimensions of the particle simulation box, the fluctuations of the shear rate obtained from the particle simulation are too large to identify a steady or oscillating shear rate as in the TB and LOB states of the model.

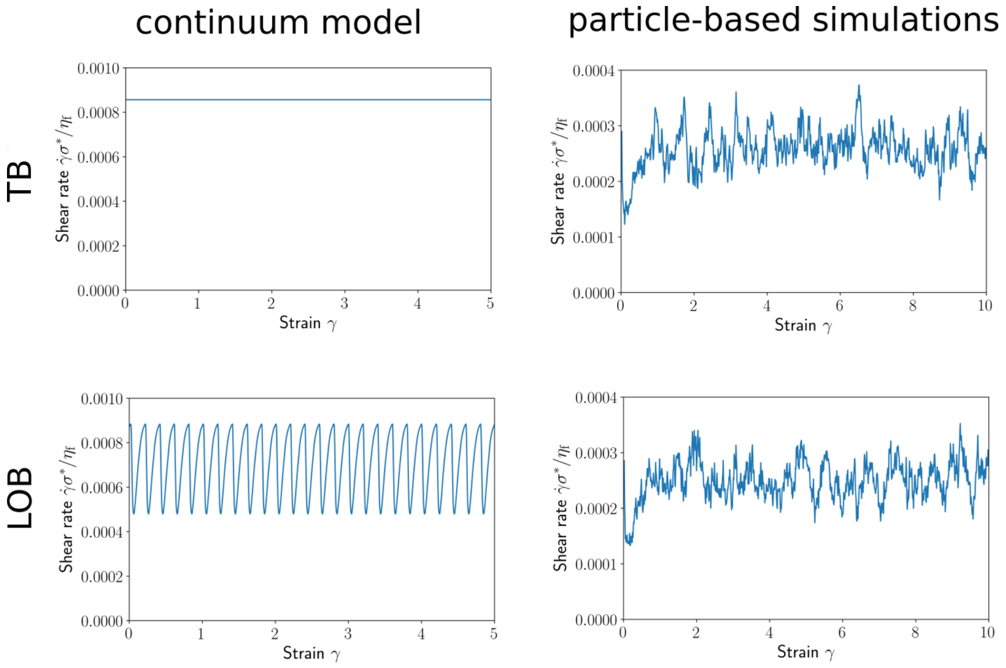


## TEST OF THE MAIN ASSUMPTIONS OF THE CONTINUUM MODEL

In this section, we verify the accuracy of the main assumptions behind our continuum model, namely Eq. 3, 4 and 5 of the main text, by comparing them with the results of the particle-based simulations.

### Fraction of frictional contacts

We first test the postulated dynamics for the fraction of frictional contacts $f$, which is defined by Eqs. 3 and 4 of the main text. We test this dynamics in the particle-based

simulations by shearing a non-banding, uniform system made of a smaller number of particles $N = 500$ in a cubic box, to ensure that the homogeneous flow remains stable. We monitor the fraction of frictional contacts computed as the ratio of contacts with $|\boldsymbol{F}_{\text{C,nor}}| > F^*$ over the total number of contacts.

*Steady-state value*

In the figure below, we test the assumed relation for the steady-state fraction of frictional contacts $f^{\text{SS}}(\sigma_{zz}) = \exp(-\sigma^*/\sigma_{zz})$ (Eq. 3 of the main text). The blue dots are the averaged values for $f$ in steady-state as a function of the applied stress from simulations with applied stresses between $0.145\sigma^*$ and $14.5\sigma^*$, a range in which shear-thickening occurs. The black line is the prediction of Eq. 3 of the main text, which shows excellent agreement with the simulation data, in line with previous studies [7].

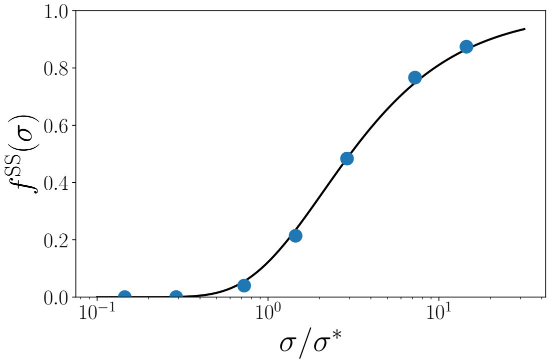


*Dynamics*

In the figure below, we test the relaxation dynamics for $f$, $\partial_t f = -\frac{\dot{\gamma}}{\gamma_0}\left[f - f^{\text{SS}}\right]$ (Eq. 4 of the main text) via the response to a step change in applied stress. Starting from an initial steady-state configuration under a stress of $3\sigma^*$, we suddenly switch the applied stress to $1.5\sigma^*$ and monitor the evolution of $f$ as a function of the applied strain $\gamma$ since the stress step. To improve the statistics, we average this response over 30 runs with independent initial configurations. The result is plotted as the blue curve in the figure below. The orange curve is an exponential relaxation with a strain $\gamma_0 = 0.023$, which is in reasonable agreement with the data. While it is clear that other values of $\gamma_0$ around 0.023 could fit the

simulation data equally well, we picked this precise value based on the fit on more accurate data of an earlier study [3].

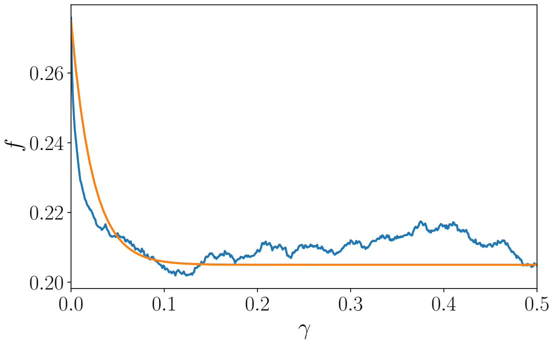


**Suspension Balance Model**

Here we test the Suspension Balance Model linking the gradient of the stress $\partial_z \sigma_{zz}$ to the velocity of the particle phase $v_z^{\mathrm{p}}$ through the linear relation $\partial_z \sigma_{zz} = -\phi\, \alpha\, v_z^{\mathrm{p}}$, which combined with mass conservation gives Eq. 5 of the main text. Naturally, we have to test this relation in a case where the stress is inhomogeneous. We do so for the simulation data shown in the top of Fig. 3 in the main text (TB state with $N = 8000$ and applied stress $\bar{\sigma} = 6.525\sigma^*$). For every time step, we generate a stress field $\sigma_{zz}(z,t)$ and velocity field $v_z^{\mathrm{p}}(z,t)$, as shown in Fig. 3 in the main text. In the figure below, we show on the right $\sigma_{zz}(z,t)$ (blue curve) and $v^{\mathrm{p}}(z,t)$ (orange curve) as a function of $z$ for a given time $t$ during the simulation. It is already apparent that indeed $v^{\mathrm{p}}$ is well correlated with $\partial_z \sigma_{zz}$. To test this relation more thoroughly, on the left we plot $\phi v_z^{\mathrm{p}}(z,t)$ as a function of $\partial_z \sigma_{zz}(z,t)$ for all $z$ and $t$ in this simulation. The data (in green circles) agree quite well with a linear relation between these two fields, and we provide the linear function in black line as a guide to the eye.

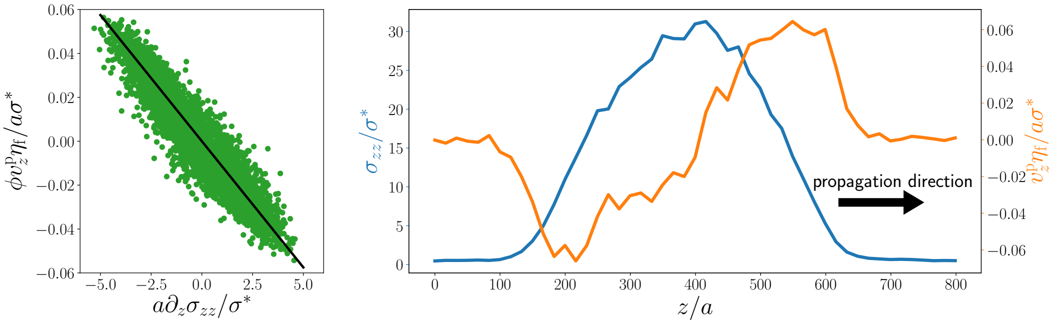

## DEPENDENCE ON BOX SIZE IN VORTICITY DIRECTION

Based on the value for the slope of the homogeneous steady state flow curve measured in smaller homogeneous simulations, our continuum model predicts an instability for systems with a vorticity length $L_z \gtrsim 200a$, which agrees fairly well with what we observe in the particle-based simulations. The data shown in the main text are for $N = 8000$ and $L_z = 815a$, but we simulated several vorticity lengths for $N = 4000$ ($L_z = 139a, 161a, 211a, 256a, 336a, 407a, 534a$) and $N = 8000$ ($L_z = 514a, 673a, 815a, 1068a$). The spatio-temporal diagrams of the fraction of frictional contacts field $f$ are shown in the figure below for $N = 4000$. For $L_z = 211a$ it is difficult to distinguish an instability from large fluctuations. However traveling bands are always unambiguously seen for $L_z = 256a$ and larger, and are not visible for $L_z = 161a$ and smaller. In order to see fully developed non linear vorticity bands, we needed to simulate systems at least twice larger than this minimal value, hence our choice of showing $L_z = 815a$ for the main text.

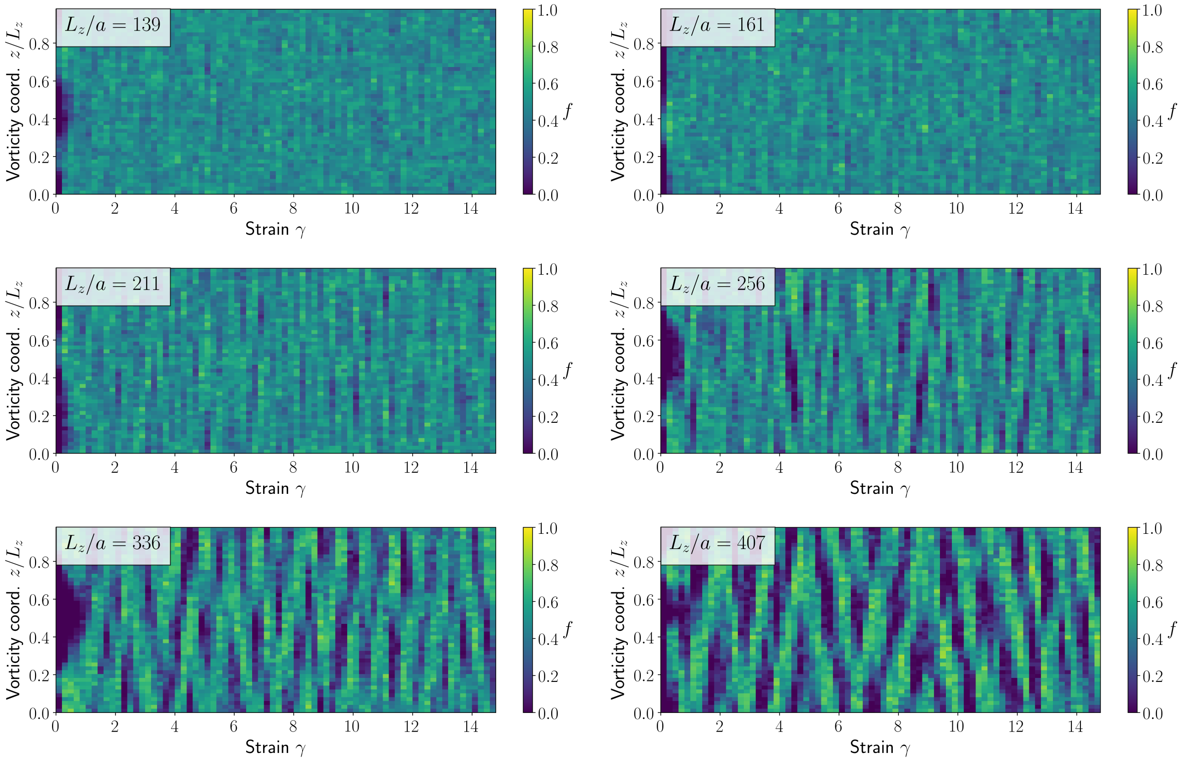

## SUPPLEMENTAL MOVIES

The spacetime plots of Fig. 3 in the main text are translated into movies to allow better visualisation of the spatio-temporal dynamics, see movies `stress_model_S6.525.mp4` and `volumefraction_model_S6.525.mp4` for Fig. 3 top left, `stress_simu_S6.525.mp4` and `volumefraction_simu_S6.525.mp4` for Fig. 3 top right, `stress_model_S7.25.mp4` and `volumefraction_model_S7.25.mp4` for Fig. 3 bottom left, `stress_simu_S7.25.mp4` and `volumefraction_simu_S7.25.mp4` for Fig. 3 bottom right.


[1] W. H. Press, S. A. Teukolsky, W. T. Vetterling, and B. P. Flannery, *Numerical Recipes 3rd Edition: The Art of Scientific Computing*, 3rd ed. (Cambridge University Press, New York, NY, USA, 2007).

[2] R. Mari, R. Seto, J. F. Morris, and M. M. Denn, J. Rheol. **58**, 1693 (2014).

[3] R. Mari, R. Seto, J. F. Morris, and M. M. Denn, Phys. Rev. E **91**, 052302 (2015).

[4] D. J. Jeffrey and Y. Onishi, Journal of Fluid Mechanics **139**, 261 (1984).

[5] M. Trulsson, B. Andreotti, and P. Claudin, Physical Review Letters **109**, 118305 (2012).

[6] D. J. Jeffrey, Physics of Fluids A: Fluid Dynamics (1989-1993) **4**, 16 (1992).

[7] A. Singh, R. Mari, M. M. Denn, and J. F. Morris, J. Rheol. **62**, 457 (2018).
